# Supplementary material for: Learning Algorithm Hyperparameters for Fast Parametric Convex Optimization
Source: arXiv:2411.15717 source file (2024-11-24)
Supplement: Supplementary file 2 [file supplement.tex]

% SIAM Supplemental File Template
\documentclass[review,supplement,onefignum,onetabnum]{siamonline220329}

\input{shared}
\usepackage{tikz}

\include{definitions}

\newif\ifpreprint
% \preprinttrue

\externaldocument[][nocite]{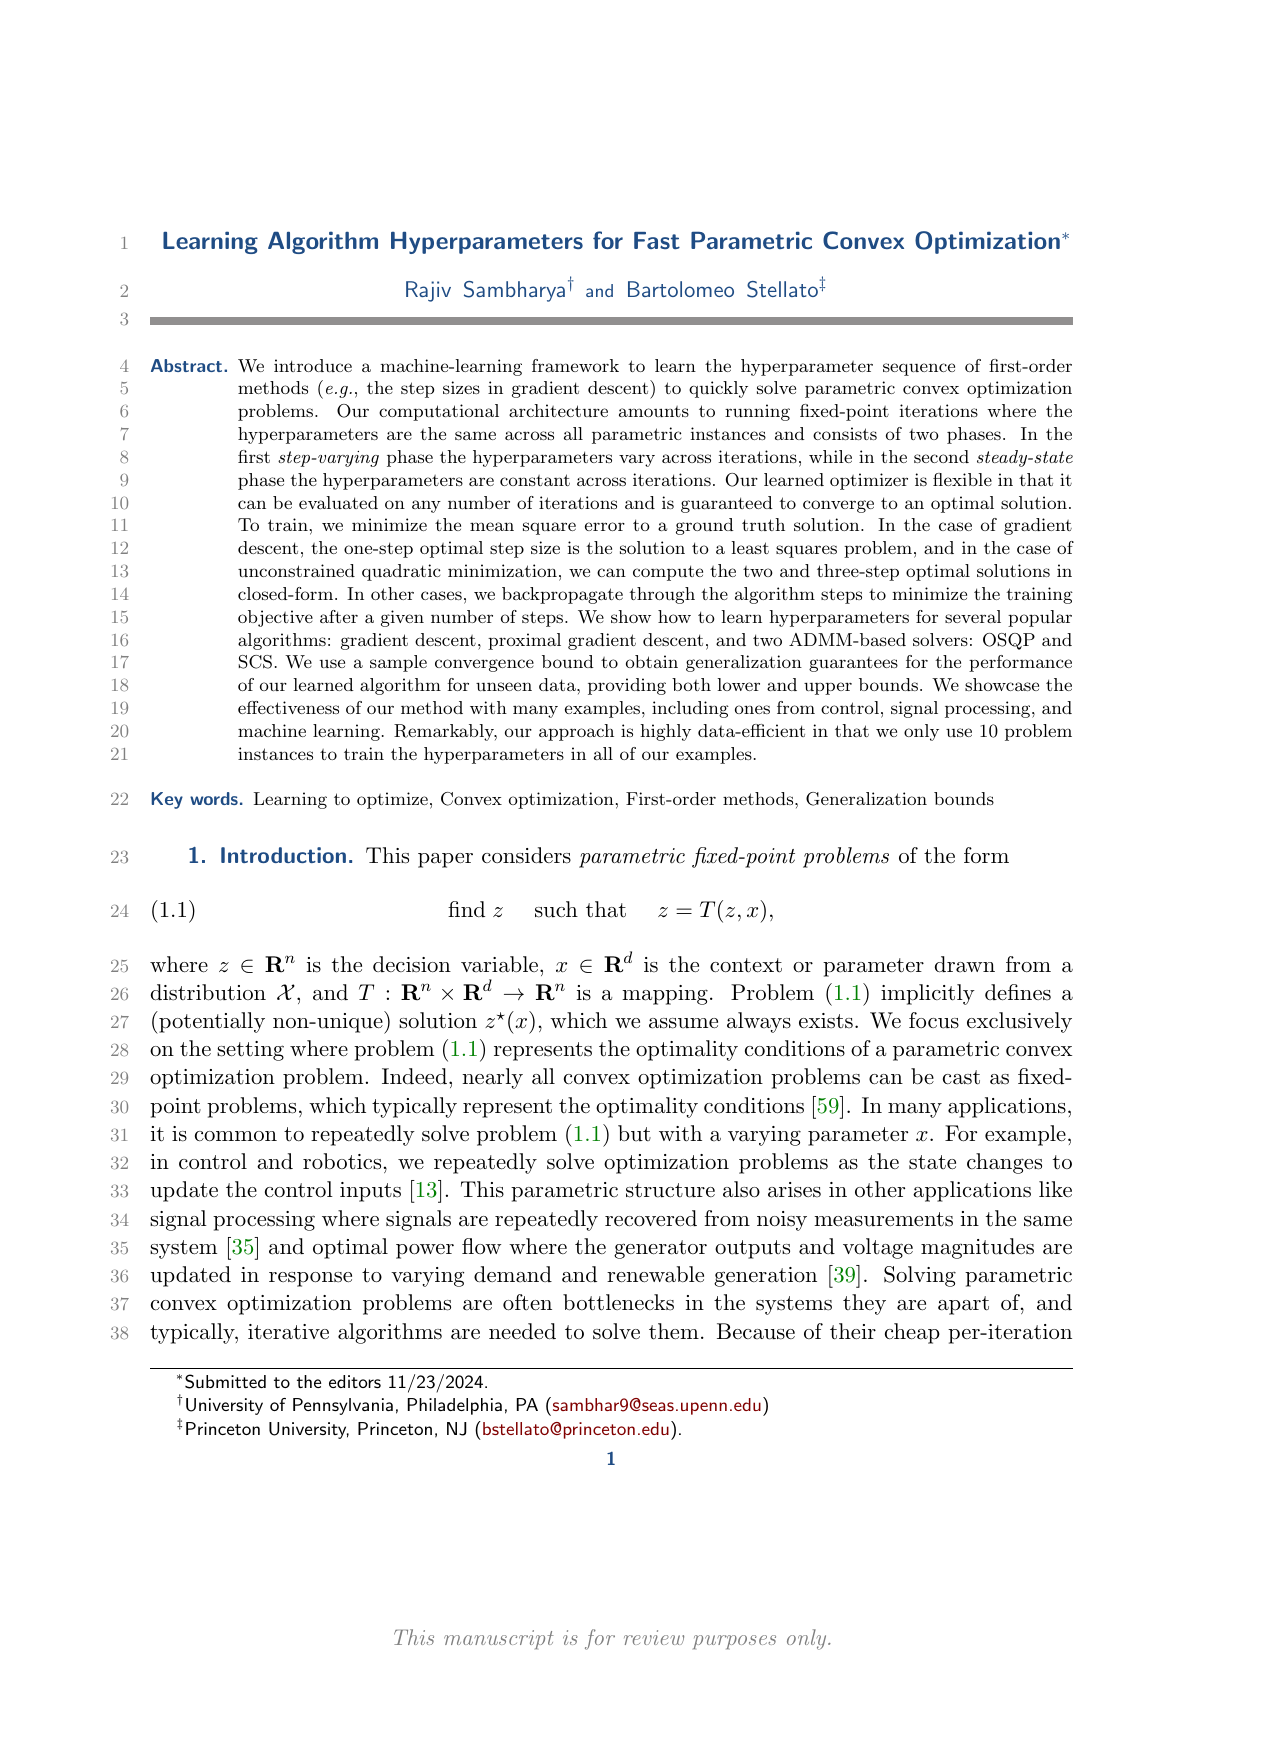}

% Optional PDF information
\ifpdf
\hypersetup{
  pdftitle={Supplementary Materials: An Example Article},
  pdfauthor={D. Doe, P. T. Frank, and J. E. Smith}
}
\fi

\begin{document}

\maketitle

\input{appendix}

\bibliographystyle{siamplain}
% \nobibliography{bibliographynourl}

\bibliography{bibliographynourl}
% \nocite{*}

\end{document}
